# Supplementary material for: Dynamic Joint Uplink and Downlink Optimization for Uplink and Downlink Decoupling-Enabled 5G Heterogeneous Networks
Source: arXiv:1607.05459 source file (2016-12-15)
Supplement: Supplementary file 1 [file appendices.tex]

\appendix
\begin{proof} 

{\it Proposition \ref{prop:Duality}:}
For any fixed BS assignment $\hat{\ve{b}}$, denote $\hW:=\ma{W}_{\hat{\ve{b}}}$ and $\hV:=\Vb$ for convenience,  the optimal downlink power solution $\hat{\ve{q}}^{\dl}$ for problem \eqref{eqn:LB_dl} satisfies \cite{stanczak2009fundamentals}
		\begin{equation}
		\vspace{-0.2em}
		\ma{\Lambda}^{\dl} \hat{\ve{q}}^{\dl}=\frac{1}{C^{\dl}(\hat{\ve{b}},\Pm)} \hat{\ve{q}}^{\dl}, \hat{\ve{q}}^{\dl}\in\R_{+}^C
		\label{eqn:DL_matrixEqua}
		\vspace{-0.2em}
		\end{equation}
		where $\ma{\Lambda}^{\dl}\in\R_{+}^{C\times C}$ is defined as
		\begin{equation}
		\vspace{-0.2em}
		\ma{\Lambda}^{\dl}:=\ma{\Gamma}\ma{\Psi}\left[\ma{A}\hV^T\Aa^T+\frac{1}{\Pm}\ve{z}^{\dl}\ve{1}_C^T\right].
		\label{eqn:DL_Lambda}
		\vspace{-0.2em}
		\end{equation}
		we denote $\ma{\Gamma}:=\diag\{\gamma_1,\ldots, \gamma_C\}$, $C^{\dl}(\hat{\ve{b}},\Pm)=\max_{\ve{q}\geq 0}\min_c U_c^{(\text{d},1)}/\gamma_c$ subject to $\|\ve{q}\|_1\leq \Pm$, and 
		$\ve{1}_C$ is a C-dimensional all-one vector.
		\eqref{eqn:DL_matrixEqua} and \eqref{eqn:DL_Lambda} are derived by writing the utility fairness $U_c^{(\text{d},1)}/\gamma_c=C^{\dl}(\hat{\ve{b}}, \Pm)$ for all $c\in\set{C}$ and the power constraint $\|\ve{q}^{\dl}\|_1=\Pm$ with matrix notation. Targets $\ve{\gamma}$ is feasible if and only if $C^{\dl}(\hat{\ve{b}},\Pm)>1$. 
		
		Similarly, the optimal uplink power solution $\hat{\ve{q}}^{\ul}$ for uplink problem \eqref{eqn:LB_ul} needs to satisfy 
		\begin{equation}
		\vspace{-0.2em}
		\ma{\Lambda}^{\ul}\hat{\ve{q}}^{\ul}=\frac{1}{C^{\ul}(\hat{\ve{b}},\Pm)} \hat{\ve{q}}^{\ul}, \hat{\ve{q}}^{\ul}\in\R_{+}^C
		\label{eqn:UL_matrixEqua}
		\vspace{-0.2em}
		\end{equation}
		where $\ma{\Lambda}^{\ul}\in\R_{+}^{C\times C}$ is defined as
		\begin{equation}
		\vspace{-0.2em}
		\ma{\Lambda}^{\ul}:=\ma{\Gamma}\ma{\Psi}\left[\ma{A}\hW\Aa^T+\frac{1}{\Pm}\ve{z}^{\ul}\ve{1}_C^T\right].
		\label{eqn:UL_Lambda}
		\vspace{-0.2em}
		\end{equation}
		where $\ve{z}^{\ul}:=\ma{A}\ve{\sigma}^{\ul}$, i.e., $z_c^{\ul}=\Sigma_{\text{tot}}/C$ for all $c\in\set{C}$. 
		
		The balanced level $C^{\dl}(\hat{\ve{b}},\Pm)$ and
		$C^{\ul}(\hat{\ve{b}},\Pm)$ are the reciprocal spectral radius of the
		nonnegative extended coupling matrix $\ma{\Lambda}^{\dl}$ and
		$\ma{\Lambda}^{\ul}$. Moreover, according to Perron-Frobenius theorem, if both $\ma{\Lambda}^{\dl}$ and
		$\ma{\Lambda}^{\ul}$ are irreducible, they have unique real spectral radius and their corresponding eigenvectors (power allocation) have strictly positive components. By comparing the interference terms in
		\eqref{eqn:DL_Lambda} and \eqref{eqn:UL_Lambda}, we have
		$(\ma{A}\hV^T\Aa^T)^T=\Aa\hV\ma{A}^T=\ma{A}\diag\{\ve{\alpha}\}\hV
		\ma{I}\ma{A}^T=\ma{A}\diag\{\ve{\alpha}\}\hV\diag^{-1}\{\ve{\alpha}\}\diag\{\ve{\alpha}\}
		\ma{A}^T=\ma{A}\hW^T\Aa^T$. By comparing the noise terms we have
		$\ve{z}^{\ul}=\frac{1}{C} \ve{1}_C{\ve{z}^{\dl}}^T\ve{1}_C$ (by using
		$z_c^{\ul}=\Sigma_{\text{tot}}/C$ for all $c\in\set{C}$), thus
		$\ve{z}^{\ul}\ve{1}_C^T=\frac{1}{C}
		\ve{1}_C{\ve{z}^{\dl}}^T\ve{1}_C\ve{1}_C^T=\ve{1}_C{\ve{z}^{\dl}}^T=(\ve{z}^{\dl}\ve{1}_C^T)^T$. By
		using the properties of spectral radius $\rho(\ma{X})=\rho(\ma{X}^T)$
		and $\rho(\ma{X}\ma{Y})=\rho(\ma{Y}\ma{X})$ we have that
		$\rho(\ma{\Lambda}^{\dl})=\rho(\ma{\Lambda}^{\ul})$ and thus
		$C^{\dl}(\hat{\ve{b}},P^{\text{max}})=C^{\ul}(\hat{\ve{b}},P^{\text{max}})$. Notice
		that the network duality holds for any given BS assignment
		$\hat{\ve{b}}$, the achievable utility regions are the same for both
		the downlink problem \eqref{eqn:LB_dl} and uplink problem
		\eqref{eqn:LB_ul}.
		\end{proof}
